# Supplementary material for: Bipartite Ranking Fairness through a Model Agnostic Ordering Adjustment
Source: arXiv:2307.14668 source file (2023-07-27)
Supplement: Supplementary file 1 [file appendix.pdf]

# Appendix of xOrder

## I. Analysis on AUC, xAUC and PRF

### A. Decomposing AUC into xAUC and iAUC

In fact, the AUC of the risk function can be decomposed into xAUC and iAUC, while iAUC means the probability of positive instances ranking above negative instances in the same group:

$$
\begin{aligned}
&\mathrm{AUC}=\frac{1}{k}\cdot\left(k_a\cdot\mathrm{iAUC}(a)+k_{a,b}\cdot\mathrm{xAUC}(a,b)+k_{b,a}\cdot\mathrm{xAUC}(b,a)+k_b\cdot\mathrm{iAUC}(b)\right)\\
&\mathrm{iAUC}(a)=\Pr\left[\mathrm{S}_1^a>\mathrm{S}_0^a\right]=\frac{1}{k_a}\sum\nolimits_{i:i\in a,\mathrm{Y}_i=1}\sum\nolimits_{j:j\in a,\mathrm{Y}_j=0}\mathbb{I}\left[R\left(\mathrm{X}_i,a\right)>R\left(\mathrm{X}_j,a\right)\right]\\
&\mathrm{iAUC}(b)=\Pr\left[\mathrm{S}_1^b>\mathrm{S}_0^b\right]=\frac{1}{k_b}\sum\nolimits_{i:i\in b,\mathrm{Y}_i=1}\sum\nolimits_{j:j\in b,\mathrm{Y}_j=0}\mathbb{I}\left[R\left(\mathrm{X}_i,b\right)>R\left(\mathrm{X}_j,b\right)\right]\\
&\mathrm{xAUC}(a,b)=\Pr\left[\mathrm{S}_1^a>\mathrm{S}_0^b\right]=\frac{1}{k_{a,b}}\cdot\sum\nolimits_{i:i\in a,\mathrm{Y}_i=1}\sum\nolimits_{j:j\in b,\mathrm{Y}_j=0}\mathbb{I}\left[R(\mathrm{X}_i,a)>R(\mathrm{X}_j,b)\right]\\
&\mathrm{xAUC}(b,a)=\Pr\left[\mathrm{S}_1^b>\mathrm{S}_0^a\right]=\frac{1}{k_{b,a}}\cdot\sum\nolimits_{i:i\in b,\mathrm{Y}_i=1}\sum\nolimits_{j:j\in a,\mathrm{Y}_j=0}\mathbb{I}\left[R(\mathrm{X}_i,b)>R(\mathrm{X}_j,a)\right]
\end{aligned}
\tag{1}
$$

in which $k_{a,b}$, $k_{b,a}$ are the same as in the main text while $k=n_0n_1$, $k_a=n_0^an_1^a$, $k_b=n_0^bn_1^b$.

### B. Analysis on PRF

From the decomposition Eq. 1, the metric of PRF can be decomposed into xAUC and iAUC as follows:

$$
\begin{aligned}
&\mathrm{PRF}(a)=\Pr[\mathrm{S}_1^a>\mathrm{S}_0]=\frac{1}{n_1^an_0}\cdot\sum\nolimits_{i:i\in a,\mathrm{Y}_i=1}\sum\nolimits_{j:\mathrm{Y}_j=0}\mathbb{I}\left[R(\mathrm{X}_i,a)>R(\mathrm{X}_j)\right]\\
&\mathrm{PRF}(b)=\Pr[\mathrm{S}_1^b>\mathrm{S}_0]=\frac{1}{n_1^bn_0}\cdot\sum\nolimits_{i:i\in b,\mathrm{Y}_i=1}\sum\nolimits_{j:\mathrm{Y}_j=0}\mathbb{I}\left[R(\mathrm{X}_i,a)>R(\mathrm{X}_j)\right]
\end{aligned}
\tag{2}
$$

According to the Eq. 1, the probability $\Pr[S_1^a>S_0]$, $\Pr[S_1^b>S_0]$ can be rewritten as follows:

$$
\begin{aligned}
&\Pr[\mathrm{S}_1^a>\mathrm{S}_0]=\frac{n_0^b}{n_0}\cdot\mathrm{xAUC}(a,b)+\frac{n_0^a}{n_0}\cdot\mathrm{iAUC}(a)\\
&\Pr[\mathrm{S}_1^b>\mathrm{S}_0]=\frac{n_0^a}{n_0}\cdot\mathrm{xAUC}(b,a)+\frac{n_0^b}{n_0}\cdot\mathrm{iAUC}(b),
\end{aligned}
\tag{3}
$$

## II. Analysis of the Transitivity of the Disparity

We will prove the proposition in the construction method. Suppose there are three groups $a$ $b$ and $c$. Each group owns three samples: $\mathrm{S}^a=\{0.61,0.71,0.72\}$, $\mathrm{S}^b=\{0.5,0.6,0.7,0.8,0.9\}$, $\mathrm{S}^c=\{0.68,0.69,0.79\}$.

We have $\Pr(\mathrm{S}^a>\mathrm{S}^b)=\frac{8}{15}>0.5$, $\Pr(\mathrm{S}^b>\mathrm{S}^c)=\frac{8}{15}>0.5$. However, $\Pr(\mathrm{S}^c>\mathrm{S}^a)=\frac{5}{9}>0.5$ holds.

## III. Proof of Proposition 1

We will prove the upper bounds about the metric $\Delta$xAUC and $\Delta$PRF in detail. For the conclusion about the metric $\Delta$URF, we could prove it in the same way.

### A. ($\Delta$xAUC)

*Proof.* Denote $T_1^a(i)=\frac{\sum_{k\le i}\mathbb{I}\left[\mathrm{Y}_{p^{a(k)}}=1\right]}{n_1^a}$, $T_1^a(i)$ is monotonically increasing on $i$ from 0 to 1. Reversely, denote $\overline{T_0^a}(i)=\frac{\sum_{k>i}\mathbb{I}\left[\mathrm{Y}_{\mathrm{p}^{a(k)}}=0\right]}{n_0^a}$ and $\overline{T_0^a}(i)$ is monotonically decreasing on $i$ from 1 to 0. Then $T_1^a(i)-\overline{T_0^a}(i)$ is monotonically increasing on $i$ from -1 to 1. So there exists an $i'$ that $T_1^a(i')-\overline{T_0^a}(i')<0$ and $T_1^a(i'+1)-\overline{T_0^a}(i'+1)\ge 0$. Since the increment of $T_1^a(i)-\overline{T_0^a}(i)$ when $i$ increases by 1 satisfies $\Delta(T_1^a(i)-\overline{T_0^a}(i))\le\max(\frac{1}{n_1^a},\frac{1}{n_0^a})$, we can get $-\max(\frac{1}{n_1^a},\frac{1}{n_0^a})\le T_1^a(i')-\overline{T_0^a}(i')<0$.

Consider a cross-group ordering which is generated by inserting the whole sequence $\mathrm{p}^b$ between $\mathrm{p}^{a(i')}$ and $\mathrm{p}^{a(i'+1)}$, this operation will result in that positive examples $\mathrm{p}^{a(k)}$ with $\mathrm{Y}_{\mathrm{p}^{a(k)}}=1, k\le i'$ will be ranked higher than all the negative examples in $\mathrm{p}^b$. And positive examples $\mathrm{p}^{a(k)}$ with $\mathrm{Y}_{\mathrm{p}^{a(k)}}=1, k>i'$ will be ranked lower than all the negative examples

in $\mathrm{p}^b$. Then $\mathrm{xAUC}(a,b)$ equals $T_1^a(i')$ with this cross-group ordering. Similarly, we can obtain $\mathrm{xAUC}(b,a) = \overline{T_0^a}(i')$. Then $\Delta\mathrm{xAUC} = |\overline{T_0^a}(i') - T_1^a(i')|$. According to the discussion above, $\Delta\mathrm{xAUC} \leq \max(\frac{1}{n_1^a}, \frac{1}{n_0^a})$.

If we consider the cross-group ordering generated by inserting the whole sequence $\mathrm{p}^a$ between $\mathrm{p}^{b(j)}$ and $\mathrm{p}^{b(j+1)}$, symmetrically we will find that there exists a corresponding $j'$ that $\Delta\mathrm{xAUC} \leq \max(\frac{1}{n_1^b}, \frac{1}{n_0^b})$ with this cross-group ordering. We can choose one of these two cross-group ordering operations to achieve $\Delta\mathrm{xAUC} \leq \min(\max(\frac{1}{n_1^b}, \frac{1}{n_0^b}), \max(\frac{1}{n_1^a}, \frac{1}{n_0^a}))$ □

### *B. (*$\Delta\mathrm{PRF}$)

*Proof.* Denote $\mathrm{C} = \frac{n_0^b}{n_0}\,\mathrm{iAUC(b)} - \frac{n_0^a}{n_0}\,\mathrm{iAUC(a)}$, we can get $-\frac{n_0^a}{n_0} \leq \mathrm{C} \leq \frac{n_0^b}{n_0}$. Since changing cross-group ordering does not affect inner-group ordering, C is constant for given $\mathrm{p}^b$ and $\mathrm{p}^a$.

With the same definition of $T_1^a(i)$ and $\overline{T_0^a}(i)$ in the Section III-A, we will have $\frac{n_0^b}{n_0}T_1^a(i) - \frac{n_0^a}{n_0}\overline{T_0^a}(i)$ is monotonically increasing on $i$ from $-\frac{n_0^a}{n_0}$ to $\frac{n_0^b}{n_0}$. Since $0 \in [-\frac{n_0^a}{n_0} - \mathrm{C}, \frac{n_0^b}{n_0} - \mathrm{C}]$, there exists $i'$ satisfying $\frac{n_0^b}{n_0}T_1^a(i') - \frac{n_0^a}{n_0}\overline{T_0^a}(i') - \mathrm{C} < 0$, $\frac{n_0^b}{n_0}T_1^a(i'+1) - \frac{n_0^a}{n_0}\overline{T_0^a}(i'+1) - \mathrm{C} \geq 0$ or $\frac{n_0^b}{n_0}T_1^a(i') - \frac{n_0^a}{n_0}\overline{T_0^a}(i') - \mathrm{C} \leq 0$, $\frac{n_0^b}{n_0}T_1^a(i'+1) - \frac{n_0^a}{n_0}\overline{T_0^a}(i'+1) - \mathrm{C} > 0$. Since the increment of $\frac{n_0^b}{n_0}T_1^a(i) - \frac{n_0^a}{n_0}\overline{T_0^a}(i) - \mathrm{C}$ when $i$ increases by 1 satisfies $\Delta(\frac{n_0^b}{n_0}T_1^a(i) - \frac{n_0^a}{n_0}\overline{T_0^a}(i) - \mathrm{C}) \leq \max(\frac{n_0^b}{n_1^a n_0}, \frac{1}{n_0})$, $-\max(\frac{n_0^b}{n_1^a n_0}, \frac{1}{n_0}) \leq \frac{n_0^a}{n_0}T_1^a(i') - \frac{n_0^b}{n_0}\overline{T_0^a}(i') - \mathrm{C} \leq \max(\frac{n_0^b}{n_1^a n_0}, \frac{1}{n_0})$.

Consider an cross-group ordering generated by inserting the whole sequence $\mathrm{p}^b$ between $\mathrm{p}^{a(i')}$ and $\mathrm{p}^{a(i'+1)}$. $\mathrm{xAUC}(a,b) = T_1^a(i')$ and $\mathrm{xAUC}(b,a) = \overline{T_0^a}(i')$. As in the calculation of $\Delta\,\mathrm{PRF} = |\frac{n_0^b}{n_0}\mathrm{xAUC}(a,b) - \frac{n_0^a}{n_0}\mathrm{xAUC}(b,a) - (\frac{n_0^b}{n_0}\,\mathrm{iAUC}(b) - \frac{n_0^a}{n_0}\,\mathrm{iAUC}(a))| = |\frac{n_0^b}{n_0}T_1^a(i') - \frac{n_0^a}{n_0}\overline{T_0^a}(i') - \mathrm{C}|$, we can get $\Delta\,\mathrm{PRF} \leq \max(\frac{n_0^b}{n_1^a n_0}, \frac{1}{n_0})$.

If we consider the cross-group ordering generated by inserting the whole sequence $\mathrm{p}^a$ between $\mathrm{p}^{b(j)}$ and $\mathrm{p}^{b(j+1)}$, symmetrically we will find there exists a corresponding $j'$ that $\Delta\,\mathrm{PRF} \leq \max(\frac{n_0^a}{n_1^b n_0}, \frac{1}{n_0})$. We can choose one from these two cross-group ordering operations and achieve $\Delta\,\mathrm{PRF} \leq \min(\max(\frac{n_0^b}{n_1^a n_0}, \frac{1}{n_0}), \max(\frac{n_0^a}{n_1^b n_0}, \frac{1}{n_0}))$. □

## IV. Analysis on Proposition 2

### *A. Proof of Proposition 2*

*Proof.* As we keep the with-in group ordering invariant, iAUC(a) and iAUC(b) remain the same after the post-processing procedure. For the objective function:

$$J(o(\mathrm{p}^a, \mathrm{p}^b)) = \mathrm{AUC}^o(o(\mathrm{p}^a, \mathrm{p}^b)) - \lambda \cdot \Delta\mathrm{xAUC}^o(o(\mathrm{p}^a, \mathrm{p}^b)) \tag{4}$$

the item $\mathrm{AUC}^o(o(\mathrm{p}^a, \mathrm{p}^b))$ can be decomposed according to Eq. 1. We subtract the constant part $k_a \cdot \mathrm{iAUC(a)}$, $k_b \cdot \mathrm{iAUC(b)}$ and multiply the formula by a constant $k$:

$$J(o(\mathrm{p}^a, \mathrm{p}^b)) = \frac{1}{k}(k_{a,b}\,\mathrm{xAUC}^o(o(\mathrm{p}^a, \mathrm{p}^b)) + k_{b,a}\,\mathrm{xAUC}^o(o(\mathrm{p}^b, \mathrm{p}^a)) - \lambda k \Delta\mathrm{xAUC}^o(o(\mathrm{p}^a, \mathrm{p}^b))) + \mathrm{C} \tag{5}$$

where C is constant $\mathrm{C} = \frac{k_a}{k} \cdot \mathrm{iAUC}(\mathrm{p}^a) + \frac{k_b}{k} \cdot \mathrm{iAUC}(\mathrm{p}^b)$

From Eq. 5, the target Eq. 4 is equivalent to:

$$\mathrm{G}(o(\mathrm{p}^a, \mathrm{p}^b)) = k_{a,b} \cdot \mathrm{xAUC}^o(o(\mathrm{p}^a, \mathrm{p}^b)) + k_{b,a} \cdot \mathrm{xAUC}^o(o(\mathrm{p}^b, \mathrm{p}^a)) - \lambda \cdot k \cdot \Delta\mathrm{xAUC}^o(o(\mathrm{p}^a, \mathrm{p}^b)). \tag{6}$$

□

Consider the definition of $\widehat{\mathrm{G}}(o(\mathrm{p}^{a(:i)}, \mathrm{p}^{b(:j)}))$ in main text Eq. (9) in which $\widehat{\mathrm{G}}(o(\mathrm{p}^{a(:i)}, \mathrm{p}^{b(:j)}))$ is induced by $\mathrm{xAUC}^o(o(\mathrm{p}^{a(:i)}, \mathrm{p}^b))$ and $\mathrm{xAUC}^o(o(\mathrm{p}^{b(:j)}, \mathrm{p}^a))$. The cross-group ordering $o(\mathrm{p}^{a(:i)}, \mathrm{p}^b)$ means appending the sequence $\mathrm{p}^{b(j+1:n^b)}$ to the given $o(\mathrm{p}^{a(:i)}, \mathrm{p}^{b(:j)})$. The meanings of partial $\mathrm{xAUC}^o(o(\mathrm{p}^{a(:i)}, \mathrm{p}^b))$ is as follows:

$$\mathrm{xAUC}^o(o(\mathrm{p}^{a(:i)}, \mathrm{p}^b)) = \frac{1}{k_{a,b}} \cdot \sum\nolimits_{k:k\leqslant i, \mathrm{Y}_{\mathrm{p}^{a(k)}}=1} \sum\nolimits_{h:h\leqslant n^b, \mathrm{Y}_{\mathrm{p}^{a(h)}}=0} \mathbb{I}\left[\mathrm{p}^{a(k)} \succ \mathrm{p}^{b(h)}\right]. \tag{7}$$

### *B. Proposition 2 and the Objective* $\widehat{\mathrm{G}}$

Considering the definition of $\widehat{\mathrm{G}}(o(\mathrm{p}^{a(:i)}, \mathrm{p}^{b(:j)}))$ in main text Eq. (9) in which $\widehat{\mathrm{G}}(o(\mathrm{p}^{a(:i)}, \mathrm{p}^{b(:j)}))$ is induced by $\mathrm{xAUC}^o(o(\mathrm{p}^{a(:i)}, \mathrm{p}^{b(:j)}) \bigoplus \mathrm{p}$ [illegible] and $\mathrm{xAUC}^o(o(\mathrm{p}^{b(:j)}, \mathrm{p}^{a(:i)}) \bigoplus \mathrm{p}^{b(j+1:n^b)})$, the cross-group ordering $o(\mathrm{p}^{a(:i)}, \mathrm{p}^{b(:j)}) \bigoplus \mathrm{p}^{b(j+1:n^b)}$ means appending the sequence $\mathrm{p}^{b(j+1:n^b)}$ to the given cross-group ordering $o(\mathrm{p}^{a(:i)}, \mathrm{p}^{b(:j)})$ ($o(\mathrm{p}^{b(:j)}, \mathrm{p}^{a(:i)}) \bigoplus \mathrm{p}^{a(i+1:n^a)}$ is similarly defined). For expression convenience, we use $o(\mathrm{p}^{a(:i)}, \mathrm{p}^b)$ to replace $o(\mathrm{p}^{a(:i)}, \mathrm{p}^{b(:j)}) \bigoplus \mathrm{p}^{b(j+1:n^b)}$, and $o(\mathrm{p}^{a(:i+1)}, \mathrm{p}^b)$ means $o(\mathrm{p}^{a(:i)}, \mathrm{p}^{b(:j)}) \bigoplus \mathrm{p}^{a(i+1)} \bigoplus \mathrm{p}^{b(j+1:n^b)}$. And the property of the partial xAUC is as follows:

$$\begin{aligned}
&\mathrm{xAUC}^o(o(\mathrm{p}^{a(:i)},\mathrm{p}^b) = \frac{1}{k_{a,b}}\cdot \sum\nolimits_{k:k\leqslant i,\mathrm{Y}_{\mathrm{p}^{a(k)}}=1}\sum\nolimits_{h:h\leqslant n^b,\mathrm{Y}_{\mathrm{p}^{a(h)}}=0}\mathbb{I}\left[\mathrm{p}^{a(k)}\succ \mathrm{p}^{b(h)}\right]\\
&\mathrm{xAUC}^o(o(\mathrm{p}^{a(:i+1)},\mathrm{p}^b) = \mathrm{xAUC}^o(o(\mathrm{p}^{a(:i)},\mathrm{p}^b) + \mathbb{I}\left[\mathrm{Y}_{\mathrm{p}^{a(i+1)}}=1\right]\cdot(\sum_{h:h>j}\mathbb{I}\left(\mathrm{Y}_{\mathrm{p}^{b(h)}}=0\right))
\end{aligned} \tag{8}$$

Obviously, when $i = n^a, j = n^b$, $\widehat{\mathrm{G}}$ equals to G in Proposition 2 of the main text.

$$\begin{aligned}
\mathrm{G}(o(\mathrm{p}^a,\mathrm{p}^b)) =& \frac{k_{a,b}}{k}\cdot \mathrm{xAUC}^o(o(\mathrm{p}^a,\mathrm{p}^b)) + \frac{k_{b,a}}{k}\cdot \mathrm{xAUC}^o(o(\mathrm{p}^b,\mathrm{p}^a))\\
&-\lambda\cdot(\mathrm{xAUC}^o(o(\mathrm{p}^a,\mathrm{p}^b)) - \mathrm{xAUC}^o(o(\mathrm{p}^b,\mathrm{p}^a)))
\end{aligned} \tag{9}$$

### C. Proposition 2 on PRF metric

The objective function under pairwise ranking fairness metric (PRF) is as follows:

$$J(o(\mathrm{p}^a,\mathrm{p}^b)) = \mathrm{AUC}^o(o(\mathrm{p}^a,\mathrm{p}^b)) - \lambda\cdot \Delta\mathrm{PRF}(o(\mathrm{p}^a,\mathrm{p}^b)) \tag{10}$$

As post-processing procedure does not change iAUC(a) and iAUC(b), the optimization target in Eq. 10 is equivalent to:

$$\begin{aligned}
&\text{Maxmizing:} \qquad \mathrm{G}(o(\mathrm{p}^a,\mathrm{p}^b))\\
&\mathrm{G}(o(\mathrm{p}^a,\mathrm{p}^b)) = k_{a,b}\cdot \mathrm{xAUC}^o(o(\mathrm{p}^a,\mathrm{p}^b)) + k_{b,a}\cdot \mathrm{xAUC}^o(o(\mathrm{p}^a,\mathrm{p}^b)) - \lambda\cdot k\cdot \Delta\mathrm{PRF}(o(\mathrm{p}^a,\mathrm{p}^b)).
\end{aligned} \tag{11}$$

## V. Proof of Theorem 1

### A. xOrder can achieve the global optimal solution of maximizing Eq.(6) in main text with $\lambda = 0$

*Proof.* We will decompose the problem that maximizing AUC into $(n^a+1)\cdot(n^b+1)$ subproblems, and $\widehat{\mathrm{G}}$ in the main text in Eq. (9) when $\lambda = 0$ is equivalent to the objective in Eq.(12). We will use mathematical induction to prove the conclusion that *xOrder can achieve the global optimal solution to maximize* $\mathrm{AUC}^o(o(\mathrm{p}^a,\mathrm{p}^b))$. For each subproblem given $i, j$ with $0\le i\le n^a, 0\le j\le n^b$, the optimization target to maximize is:

$$\begin{aligned}
\widehat{\mathrm{G}}(o(\mathrm{p}^{a(:i)},\mathrm{p}^{b(:j)})) = &\sum\nolimits_{k:k\leqslant i,\mathrm{Y}_{\mathrm{p}^{a(k)}}=1}\sum\nolimits_{h:h\leqslant n^b,\mathrm{Y}_{\mathrm{p}^{b(h)}}=0}\mathbb{I}\left[\mathrm{p}^{a(k)}\succ \mathrm{p}^{b(h)}\right]+\\
&\sum\nolimits_{k:k\leqslant n^a,\mathrm{Y}_{\mathrm{p}^{a(k)}}=0}\sum\nolimits_{h:h\leqslant j,\mathrm{Y}_{\mathrm{p}^{b(h)}}=1}\mathbb{I}\left[\mathrm{p}^{b(h)}\succ \mathrm{p}^{a(k)}\right]
\end{aligned} \tag{12}$$

For any $0\le i\le n_a, 0\le j\le n_b$, according to the property in Eq. 13, the update equation when $\mathrm{p}^{a(:i+1)}$ is appended to $o(\mathrm{p}^{a(:i)},\mathrm{p}^{b(:j)})$:

$$\widehat{\mathrm{G}}(o(\mathrm{p}^{a(:i)},\mathrm{p}^{b(:j)})\bigoplus \mathrm{p}^{a(:i+1)}) = \widehat{\mathrm{G}}(o(\mathrm{p}^{a(:i)},\mathrm{p}^{b(:j)})) + \mathbb{I}\left[\mathrm{Y}_{\mathrm{p}^{a(i+1)}}=1\right]\cdot(\sum_{h:h>j}\mathbb{I}\left(\mathrm{Y}_{\mathrm{p}^{b(h)}}=0\right)). \tag{13}$$

Consider two trivial cases of $o(\mathrm{p}^{a(:0)},\mathrm{p}^{b(:j)})$ $(0<j\le n^b)$ and $o(\mathrm{p}^{a(:i)},\mathrm{p}^{b(:0)})$ $(0<i\le n^a)$, there is only one possible path. The unique solution is obtained at the initialized stage of `xOrder` algorithm.

For any given $i$ and $j$ satisfying $i>0$ and $j>0$, suppose `xOrder` has got the optimal solutions $o^*(\mathrm{p}^{a(:i-1)},\mathrm{p}^{b(:j)})$ and $o^*(\mathrm{p}^{a(:i)},\mathrm{p}^{b(:j-1)}))$ of the subproblems to maximize $\widehat{\mathrm{G}}(o(\mathrm{p}^{a(:i-1)},\mathrm{p}^{b(:j)}))$ and $\widehat{\mathrm{G}}(o(\mathrm{p}^{a(:i)},\mathrm{p}^{b(:j-1)}))$ respectively.

Now, we will prove the solution $o^*(\mathrm{p}^{a(:i)},\mathrm{p}^{b(:j)})$ returned by `xOrder` is optimal by contradiction. Suppose there exists $\overline{o}(\mathrm{p}^{a(:i)},\mathrm{p}^{b(:j)})$ satisfying $\widehat{\mathrm{G}}(\overline{o}(\mathrm{p}^{a(:i)},\mathrm{p}^{b(:j)})) > \widehat{\mathrm{G}}(o^*(\mathrm{p}^{a(:i)},\mathrm{p}^{b(:j)}))$. There are two possible situations: $\overline{o}(\mathrm{p}^{a(:i)},\mathrm{p}^{b(:j)})$ ends with 1).$\mathrm{p}^{a(i)}$, 2).$\mathrm{p}^{b(j)}$. Without the loss of generality, we assume $\overline{o}(\mathrm{p}^{a(:i)},\mathrm{p}^{b(:j)})$ ends with $\mathrm{p}^{a(i)}$ and define $\overline{o}(\mathrm{p}^{a(:i-1)},\mathrm{p}^{b(:j)})$ by $\overline{o}(\mathrm{p}^{a(:i)},\mathrm{p}^{b(:j)}) = \overline{o}(\mathrm{p}^{a(:i-1)},\mathrm{p}^{b(:j)})\bigoplus \mathrm{p}^{a(i)}$. We can get the following inequation:

$$\begin{aligned}
&\widehat{\mathrm{G}}(\overline{o}(\mathrm{p}^{a(:i-1)},\mathrm{p}^{b(:j)})) = \widehat{\mathrm{G}}(\overline{o}(\mathrm{p}^{a(:i)},\mathrm{p}^{b(:j)})) - \mathbb{I}\left[\mathrm{Y}_{\mathrm{p}^{a(i)}}=1\right]\cdot(\sum_{h:h>j}\mathbb{I}\left(\mathrm{Y}_{\mathrm{p}^{b(h)}}=0\right))\\
&>\widehat{\mathrm{G}}(o^*(\mathrm{p}^{a(:i)},\mathrm{p}^{b(:j)})) - \mathbb{I}\left[\mathrm{Y}_{\mathrm{p}^{a(i)}}=1\right]\cdot(\sum_{h:h>j}\mathbb{I}\left(\mathrm{Y}_{\mathrm{p}^{b(h)}}=0\right))\\
&\ge \widehat{\mathrm{G}}(o^*(\mathrm{p}^{a(:i-1)},\mathrm{p}^{b(:j)})\bigoplus \mathrm{p}^{a(i)}) - \mathbb{I}\left[\mathrm{Y}_{\mathrm{p}^{a(i)}}=1\right]\cdot(\sum_{h:h>j}\mathbb{I}\left(\mathrm{Y}_{\mathrm{p}^{b(h)}}=0\right)),\\
&=\widehat{\mathrm{G}}(o^*(\mathrm{p}^{a(:i-1)},\mathrm{p}^{b(:j)}))
\end{aligned} \tag{14}$$

where $\ge$ in the third line holds due to the update process of `xOrder` in the main text Eq. (8). This violates the assumption that $o^*(\mathrm{p}^{a(:i-1)},\mathrm{p}^{b(:j)}))$ is optimal. For the situation that $\overline{o}(\mathrm{p}^{a(:i)},\mathrm{p}^{b(:j)})$ ends with $\mathrm{p}^{b(j)}$, similarly we can derive

$\widehat{\mathrm{G}}(\overline{o}(\mathrm{p}^{a(:i)}, \mathrm{p}^{b(:j-1)})) > \widehat{\mathrm{G}}(o^*(\mathrm{p}^{a(:i)}, \mathrm{p}^{b(:j-1)}))$, which violates the assumption $o^*(\mathrm{p}^{a(:i)}, \mathrm{p}^{b(:j-1)}))$ is optimal. Summarizing the deduction above, we can get $o^*(\mathrm{p}^{a(:i)}, \mathrm{p}^{b(:j)})$ must be optimal.

Due to the generality of $i$ and $j$, $o^*(\mathrm{p}^a, \mathrm{p}^b)$ with $i = n^a$ and $j = n^b$ is the global optimal solution to maximize $\mathrm{AUC}^o(o(\mathrm{p}^a, \mathrm{p}^b))$. □

For the objective in the following Eq. (15) with $\lambda > 0$, `xOrder` could also achieve the global optimal solution. The proof is similar to the above, which is proved by contradiction,

$$\mathrm{J}(o(\mathrm{p}^a, \mathrm{p}^b)) = \mathrm{AUC}^o(o(\mathrm{p}^a, \mathrm{p}^b)) - \lambda(\mathrm{xAUC}^o(o(p^a, p^b)) - \mathrm{xAUC}^o(o(p^b, p^a))). \quad (15)$$

*B. xOrder has the upper bounds of fairness disparities stated in Eq.(10) in the main text as $\lambda$ approaches infinity*

In the beginning, we will prove that `xorder` has the disparity upper bound $\Delta\mathrm{xAUC} \le \max\left(\frac{1}{n_1^a}, \frac{1}{n_1^b}\right)$. We also decompose the problem in Eq.(6) into $(n^a+1)\cdot(n^b+1)$ subproblems as the last proof does. As $\lambda$ approaches infinity, maximizing the objective in Eq.(9) means minimizing $\Delta\mathrm{xAUC}$ exactly and is equivalent to maximizing the objective in Eq.(16).

$$\begin{aligned}&\widehat{\mathrm{G}}(o(\mathrm{p}^{a(:i-1)}, \mathrm{p}^{b(:j)})) = -\left|\widehat{\mathrm{H}}(o(\mathrm{p}^{a(:i-1)}, \mathrm{p}^{b(:j)}))\right| \\ &\widehat{\mathrm{H}}(o(\mathrm{p}^{a(:i-1)}, \mathrm{p}^{b(:j)})) = \sum\nolimits_{k:k\leqslant i, \mathrm{Y}_{\mathrm{p}^{a(k)}}=1} \sum\nolimits_{h:h\leqslant n^b, \mathrm{Y}_{\mathrm{p}^{b(h)}}=0} \mathbb{I}\left[\mathrm{p}^{a(k)} \succ \mathrm{p}^{b(h)}\right] - \\ &\sum\nolimits_{k:k\leqslant n^a, \mathrm{Y}_{\mathrm{p}^{a(k)}}=0} \sum\nolimits_{h:h\leqslant j, \mathrm{Y}_{\mathrm{p}^{b(h)}}=1} \mathbb{I}\left[\mathrm{p}^{b(h)} \succ \mathrm{p}^{a(k)}\right]\end{aligned} \quad (16)$$

**Definition 1** (greedy forward search algorithm). *For any $0 \le i \le n^a$, $0 \le j \le n^b$, given $\overline{o}(\mathrm{p}^{a(:i)}, \mathrm{p}^{b(:j)})$, the update function of the greedy forward search algorithm is as follows:*

$$\begin{aligned}&\textit{Given} \quad o^*(\mathrm{p}^{a(:i)}, \mathrm{p}^{b(:j)}) \\ &\textit{if:}\ \widehat{\mathrm{G}}(o^*(\mathrm{p}^{a(:i)}, \mathrm{p}^{b(:j)}) \bigoplus \mathrm{p}^{a(i+1)}) \ge \widehat{\mathrm{G}}(o^*(\mathrm{p}^{a(:i)}, \mathrm{p}^{b(:j)}) \bigoplus \mathrm{p}^{b(j+1)}) \\ &\quad \textit{update:} \quad o^*(\mathrm{p}^{a(:i+1)}, \mathrm{p}^{b(:j)}) = o^*(\mathrm{p}^{a(:i)}, \mathrm{p}^{b(:j)}) \bigoplus \mathrm{p}^{a(i+1)}; \\ &\textit{otherwise:} \\ &\quad \textit{update:} \quad o^*(\mathrm{p}^{a(:i)}, \mathrm{p}^{b(:j+1)}) = o^*(\mathrm{p}^{a(:i)}, \mathrm{p}^{b(:j)}) \bigoplus \mathrm{p}^{b(j+1)},\end{aligned} \quad (17)$$

Using the algorithm defined above, we can find an optimal path to minimize the xAUC disparity in a greedy manner.

**Lemma 1.** *greedy search forward algorithm can achieve the upper bound $\Delta\mathrm{xAUC} \le \max\left(\frac{1}{n_1^a}, \frac{1}{n_1^b}\right)$.*

*Proof.* We will use mathematical induction to prove the lemma. As $i = 0$ and $j = 0$, without loss of generality, we assume $\widehat{\mathrm{G}}(o^*(\mathrm{p}^{a(:0)}, \mathrm{p}^{b(:0)}) \bigoplus \mathrm{p}^{a(1)}) \ge \widehat{\mathrm{G}}(o^*(\mathrm{p}^{a(:0)}, \mathrm{p}^{b(:0)}) \bigoplus \mathrm{p}^{b(1)})$, then following the update function in Eq.(17) we get $\widehat{\mathrm{G}}(o^*(\mathrm{p}^{a(:i)}, \mathrm{p}^{b(:j)}) \ge -\min(\frac{1}{n_1^a}, \frac{1}{n_1^b}) \ge -\max(\frac{1}{n_1^a}, \frac{1}{n_1^b})$. Without loss of generality, suppose there exists $\widehat{\mathrm{H}}(o^*(\mathrm{p}^{a(:i)}, \mathrm{p}^{b(:j)}) \le \max(\frac{1}{n_1^a}, \frac{1}{n_1^b})$ while $\widehat{\mathrm{H}}(o^*(\mathrm{p}^{a(:i+1)}, \mathrm{p}^{b(:j)}) = \widehat{\mathrm{H}}(o^*(\mathrm{p}^{a(:i)}, \mathrm{p}^{b(:j)}) + \mathbb{I}\left[\mathrm{Y}_{\mathrm{p}^{a(i+1)}} = 1\right] \cdot \left(\sum_{h:h\le n^b} \mathbb{I}\left(\mathrm{Y}_{\mathrm{p}^{b(h)}} = 0\right)\right) > \max(\frac{1}{n_1^a}, \frac{1}{n_1^b})$ after the next update. As $\mathrm{p}^{a(i+1)})$ is appended to $o^*(\mathrm{p}^{a(:i)}, \mathrm{p}^{b(:j)})$ following the update function Eq.(17), we can conclude that $\widehat{\mathrm{H}}(o^*(\mathrm{p}^{a(:i)}, \mathrm{p}^{b(:j)}) > 0$ and

$$\max(\frac{1}{n_1^a}, \frac{1}{n_1^b}) < \widehat{\mathrm{H}}(o^*(\mathrm{p}^{a(:i+1)}, \mathrm{p}^{b(:j)})) \le -\widehat{\mathrm{G}}(o^*(\mathrm{p}^{a(:i)}, \mathrm{p}^{b(:j+1)})). \quad (18)$$

As $0 \le \widehat{\mathrm{H}}(o^*(\mathrm{p}^{a(:i)}, \mathrm{p}^{b(:j)})) \le \max(\frac{1}{n_1^a}, \frac{1}{n_1^b})$, $0 \le \mathbb{I}\left[\mathrm{Y}_{\mathrm{p}^{b(j+1)}} = 1\right] \cdot (\sum_{h:h>i} \mathbb{I}\left(\mathrm{Y}_{\mathrm{p}^{a(h)}} = 0\right)) \le \max(\frac{1}{n_1^a}, \frac{1}{n_1^b})$, $-\widehat{\mathrm{G}}(o^*(\mathrm{p}^{a(:i)}, \mathrm{p}^{b(:j+1)})) = \left|\widehat{\mathrm{H}}(o^*(\mathrm{p}^{a(:i)}, \mathrm{p}^{b(:j+1)}))\right| = \left|\widehat{\mathrm{H}}(o^*(\mathrm{p}^{a(:i)}, \mathrm{p}^{b(:j)})) - \mathbb{I}\left[\mathrm{Y}_{\mathrm{p}^{b(j+1)}} = 1\right] \cdot (\sum_{h:h\le n^a} \mathbb{I}\left(\mathrm{Y}_{\mathrm{p}^{a(h)}} = 0\right))\right| \le \max(\frac{1}{n_1^a}, \frac{1}{n_1^b})$. This violates the conclusion in Eq.(18), thus we prove that $-\widehat{\mathrm{G}}(o^*(\mathrm{p}^{a(:n^a)}, \mathrm{p}^{b(:n^b)})) = \Delta\mathrm{xAUC} \le \max\left(\frac{1}{n_1^a}, \frac{1}{n_1^b}\right)$ using greedy forward update algorithm. □

**Lemma 2.** *The upper bound of $\Delta\mathrm{xAUC}$ achieved by the greedy search forward algorithm is no less than `xorder`.*

*Proof.* We also use mathematical induction to prove the lemma. We use $_{\#greedy}\widehat{\mathrm{G}}$ and $_{\#xorder}\widehat{\mathrm{G}}$ to represent the value of $\widehat{\mathrm{G}}$ defined in Eq.(16) obtained by *greedy search forward algorithm* and `xorder`, respectively. As $i = 0$ and $j = 0$, there exists $0 =_{\#greedy} \widehat{\mathrm{G}}(o^*(\mathrm{p}^{a(:0)}, \mathrm{p}^{b(:0)})) \le_{\#xorder} \widehat{\mathrm{G}}(o^*(\mathrm{p}^{a(:0)}, \mathrm{p}^{b(:0)})) = 0$. Suppose $_{\#greedy}\widehat{\mathrm{G}}(o^*(\mathrm{p}^{a(:i)}, \mathrm{p}^{b(:j)})) \le_{\#xorder} \widehat{\mathrm{G}}(o^*(\mathrm{p}^{a(:i)}, \mathrm{p}^{b(:j)}))$, without loss of generality, we assume $\mathrm{p}^{a(i+1)}$ is appended to $o^*(\mathrm{p}^{a(:i)}, \mathrm{p}^{b(:j)})$ following the update function

TABLE I: Running time comparisons with two groups (seconds)

| Dataset | post-logit | corr-reg | opti-tfco | xOrder |
|---|---|---|---|---|
| COMPAS | 0.288 | 1.191 | 26.306 | 2.356 |
| Adult | 0.446 | 4.775 | 280.631 | 31.443 |
| large eICU | 1.285 | 16.526 | >86400 | 1383.106 |

TABLE II: Running time comparisons with different numbers of sample size on large eICU (seconds)

| Sample size | 2000 | 4000 | 8000 | 16000 | 32000 | 64000 |
|---|---|---|---|---|---|---|
| Running-time | 0.745 | 1.446 | 6.211 | 31.920 | 196.353 | 1331.732 |

Eq.(17). Now we will prove that ${}_{\#greedy}\widehat{\mathrm{G}}(o^*(\mathrm{p}^{a(:i+1)},\mathrm{p}^{b(:j)})) \leq_{\#xorder} \widehat{\mathrm{G}}(o^*(\mathrm{p}^{a(:i+1)},\mathrm{p}^{b(:j)}))$. From Eq.(8) in the main text, we get the following inequation:

$$\begin{aligned} {}_{\#xorder}\widehat{\mathrm{G}}(o^*(\mathrm{p}^{a(:i+1)},\mathrm{p}^{b(:j)})) &= \max\left({}_{\#xorder}\widehat{\mathrm{G}}(o^*(\mathrm{p}^{a(:i)},\mathrm{p}^{b(:j)})\bigoplus \mathrm{p}^{a(i+1)}, {}_{\#xorder}\widehat{\mathrm{G}}(o^*(\mathrm{p}^{a(:i+1)},\mathrm{p}^{b(:j-1)})\bigoplus \mathrm{p}^{b(j)})\right) \\ &\geq \max\left({}_{\#greedy}\widehat{\mathrm{G}}(o^*(\mathrm{p}^{a(:i)},\mathrm{p}^{b(:j)})\bigoplus \mathrm{p}^{a(i+1)}, {}_{\#xorder}\widehat{\mathrm{G}}(o^*(\mathrm{p}^{a(:i+1)},\mathrm{p}^{b(:j-1)})\bigoplus \mathrm{p}^{b(j)})\right) \\ &\geq_{\#greedy} \widehat{\mathrm{G}}(o^*(\mathrm{p}^{a(:i)},\mathrm{p}^{b(:j)})\bigoplus \mathrm{p}^{a(i+1)} \\ &\geq_{\#greedy} \widehat{\mathrm{G}}(o^*(\mathrm{p}^{a(:i+1)},\mathrm{p}^{b(:j)})) \end{aligned} \tag{19}$$

where the $\geq$ in the second line holds due to our assumption that ${}_{\#greedy}\widehat{\mathrm{G}}(o^*(\mathrm{p}^{a(:i)},\mathrm{p}^{b(:j)})) \leq_{\#xorder} \widehat{\mathrm{G}}(o^*(\mathrm{p}^{a(:i)},\mathrm{p}^{b(:j)}))$. Summarizing the deduction above, we get that ${}_{\#greedy}\widehat{\mathrm{G}}(o^*(\mathrm{p}^{a(:n^a)},\mathrm{p}^{b(:n^b)})) \leq_{\#xorder} \widehat{\mathrm{G}}(o^*(\mathrm{p}^{a(:n^a)},\mathrm{p}^{b(:n^b)}))$. Recalling that $\widehat{\mathrm{G}}(o^*(\mathrm{p}^{a(:n^a)},\mathrm{p}^{b(:n^b)})) = -\Delta\mathrm{xAUC}$, we prove that the upper bound of $\Delta$xAUC achieved by greedy search forward algorithm is no less than `xorder`. □

Combining the two lemmas above, we prove that `xorder` achieves that $\Delta\mathrm{xAUC} \leq \max\left(\frac{1}{n_1^a}, \frac{1}{n_1^b}\right)$ as $\lambda$ approaches infinity. For the proposition that `xorder` achieves that $\Delta\mathrm{URF} \leq \max\left(\frac{1}{n^a}, \frac{1}{n^b}\right)$ and $\Delta\mathrm{PRF} \leq \max\left(\frac{n_0^b}{n_0 \cdot n_1^a}, \frac{n_0^a}{n_0 \cdot n_1^b}\right)$ as $\lambda$ approaches infinity, we can prove it in a similar way.

## VI. Time Complexity and Memory Requirement Analysis

### A. Time Complexity

In this section, we analyze the time complexity of `xOrder` and baselines and provide running-time comparisons on different datasets. Suppose there are $K$ groups and each group has $N$ samples, where are $N/2$ positive samples and $N/2$ negative samples, note that the computation complexity of AUC is $O(N \log N)$

1) **post-logit:** post-logit exhaustively tries all parameters of the transformation function, and looks for the optimal parameter with the lowest disparity. It only needs to compute the disparities of each pair of groups, which has the time complexity $O(K^2 N \log N)$. Therefore, the time complexity is $O(K^2 N \log N)$.
2) **corr-reg:** corr-reg proposes to learn a fair ranking which uses a regularizer for each pair of groups. So it has $K^2$ regularizers. For the objective computation, it needs to compute the prediction loss ($O(N)$), the regularizers ($O(K^2 N \log N)$). Therefore, the time complexity is $O(K^2 N \log N)$.
3) **xOrder:** the optimization process of iterative `xOrder` is $O(N^2)$ for two groups. Since the iterative `xOrder` needs to optimize $K-1$ times for $K$ groups, and the $i-$th optimization is to find the optimal path for the aggregated group with $(K-1)N$ samples and the $K+1$ group with $N$ samples. Therefore, the final time complexity is $O(K^2N^2) = O(N^2 + 2*N^2+, ..., +(K-1)*N^2)$. When the number of samples veries in different groups (e.g., the $i$-th groups has 2000 samples but the $j$-th groups has 3000 samples), the time complexity is is $O(K^2 N_{max}^2)$, where $N_{max}$ denotes the maximum of the sample size of all groups.

For the running-time comparisons, we first compare all baselines on Adult, COMPAS and large eICU dataset with two groups, and the results are shown in Table I.

For the experiments on the dataset large eICU, we tried many hyperparameter combinations for opti-tfco following the setting stated in Appendix in [1], but still could not get a converged result within 48 hours. We guess that the framework opti-tfco learning a solution satisfying the constraints strictly needs to run so many rounds. From Table I, post-logit has the minimum time cost. opti-tfco has the maximum time cost for a converged solution satisfying the fairness constraints.

Then, we report the running-times of `xOrder` with different number of sample size on the dataset large eICU with two groups. The results are shown in Table II. From Table II, the running-time and the square of sample size are proportional.

For the running-time with multiple protected groups, we conduct experiments on large eICU with 2, 5, and 10 protected groups. The running-time results are shown in Table III.

For the dataset large eICU, more protected groups $K$ means less sample size in each group $N$. Since $K*N$ is constant and the time complexity of `xOrder` is $O(K^2N^2)$, `xOrder` has similar running-time when the number of protected groups

TABLE III: Running time comparisons with the different number of protected groups on large eICU (seconds)

| Groups | post-logit | corr-reg | opti-tfco | xOrder |
|---|---|---|---|---|
| 2 | 1.285 | 16.526 | >86400 | 1383.106 |
| 5 | 3.280 | 303.550 | >86400 | 3407.797 |
| 10 | 8.871 | 430.493 | >86400 | 3338.725 |

is 5 and 10 shown in Table III. When there are two protected groups, it does not need to iterate the ordering of the groups. So it has less running-time cost as in Table III.

### B. Memory Requirment Analysis

Suppose there are $K$ groups and each group has $N$ samples, the memory requirement of `xOrder` is $O(KN)$ for computing $\widehat{\mathrm{G}}\left(o^*\left(\mathrm{p}^{a(:i)}, \mathrm{p}^{b(:j)}\right)\right)$ shown in Figure 3 in the maintext. From Figure 3 in the maintext, we compute the ordering $o(p^{a(:i)}, p^{b(:j)})$ only using $o(p^{a(:i-1)}, p^{b(:j)})$ and $o(pa(:i), pb(:j-1))$, which means that `xOrder` does not need to save all $o(p^{a(:m)}, p^{b(:n)}), (m = 1, ..., n^a, n = 1, ..., n^b)$.

In the implementation, for two protected groups, compute the ordering $o(p^{a(:i)}, p^{b(:j)})$, xorder only saves $o(p^{a(:i-1)}, p^{b(:n)}), (n = 1, ..., n^b)$ and $o(p^{a(:m)}, p^{b(:j-1)}), (m = 1, ..., n^a)$. Meanwhile, the memory requirement of $o(p^{a(:i-1)}, p^{b(:n)}), (n = 1, ..., n^b)$ (or $o(p^{a(:m)}, p^{b(:j-1)}), (m = 1, ..., n^a)$) is $O(2 * N^2)$. Therefore, the memory requirement is $O(2 * N^2)$. For $K$ protected groups, the memory requirement of iterative xOrder is $O(KN^2)$, which is acceptable in most real ranking scenarios.

## VII. Implementation details

### A. Data preprocess

For the four fairness benchmark data sets, we use the preprocessed data sets from the resource of [2], while three of them(COMPAS, Adult) are from the resource of [3]. All categorical variables will be encoded as one-hot features. For Framingham, we use all features as the input. For MIMIC-III data set, we preprocess the original data as in [4] for each ICU admission. EHR data of 17 selected clinical variables from the first 48 hours are used to extract features. For all clinical variables, different statistics (mean, std, etc) of different time slices are extracted to form a vector with 714 features.

### B. Training process of model

We first train a model without any fairness regularization to obtain the unadjusted result. The linear model is optimized by gradient descent with learning rate of 1.0 and tfco respectively. The model is trained for at most 100 epochs. If the training loss failed to reduce after 5 consecutive epochs, the training will be stopped. For bipartite rankboost model, the number of estimators is 50 and learning rate is 1.0, which are the same as in the experiments of [2].

**Post-logit** With transformation function $f(x) = \frac{1}{1+e^{-(\alpha x+\beta)}}$, We follow the same procedure in [2] to optimize empirical disparity($\Delta\mathrm{xAUC}$ or $\Delta\mathrm{PRF}$) with fixed $\beta = -2$. The value of $\alpha$ is chosen from $[0, 10]$. However, we find that this setting can not obtain equal $\mathrm{xAUC}$ or $\mathrm{PRF}$ in MIMIC data set which has not been used in [2]. So we change $\beta$ from $[-1, -3]$ and $\alpha$ from $[0, 10]$ when optimizing the empirical disparity on MIMIC data set. As this method cannot be directly used for the setting with three protected groups $a$, $b$, and $c$, we iteratively calibrate the ranking scores from group $b$ and $c$.

**Corr-reg** For corr-reg, we train models of the same structure with various weights of fairness regularization. Since the correlation regularization is only an approximation of the pairwise ranking disparity, we use the corresponding ranking fairness metrics($\Delta\mathrm{xAUC}$ or $\Delta\mathrm{PRF}$) as the criterion to determine the range of weights. We initialize the weight to be 0 (equivalent to unadjusted) and increase it until the average ranking disparity on training data is lower than $0.0001$ or does not decrease in 2 consecutive steps. We also apply this strategy to `xOrder`.

**Opti-tfco** For opti-tfco, we use the implementation of [1]. When considering the trade-off between utility and fairness in a bipartite ranking problem, the authors optimize a constrained problem which is defined as follows: the model is trained to maximize AUC under the constrain that disparity($\Delta\mathrm{xAUC}$ or $\Delta\mathrm{PRF}$) is smaller than hyper-parameter $\epsilon$.

### C. Computing infrastructure and consumption

We run `xOrder` on the computer with Intel i7-9750H CPU(@2.6GHz $\times$ 6) and 16 GB RAM.

## VIII. Robustness Discussion

### A. Fewer Training Samples

To assess the performance of our algorithm given fewer training samples, we conduct the experiments with a different number of training samples, in which we select a linear model as the base model with the optimization framework in [1]. From Figure 1(a), as the number of training samples changed from 4000 to 1000, `xOrder` achieves a lower disparity compared to baselines. Meanwhile, `xOrder` still achieves a lower disparity while maintaining a maximum algorithm utility. Experiment

TABLE IV: Summary of ranking fairness metrics on unadjusted result over 10 repeat experiments

| Data set | Linear Model(gradient descent) | | Linear Model(AUC) | | Bipartite Rankboost | |
|---|---|---|---|---|---|---|
| | ΔxAUC | ΔPRF | ΔxAUC | ΔPRF | ΔxAUC | ΔPRF |
| COMPAS | $0.195 \pm 0.024$ | $0.119 \pm 0.015$ | $0.220 \pm 0.026$ | $0.138 \pm 0.019$ | $0.206 \pm 0.027$ | $0.134 \pm 0.019$ |
| Adult | $0.089 \pm 0.011$ | $0.040 \pm 0.009$ | $0.086 \pm 0.010$ | $0.034 \pm 0.008$ | $0.055 \pm 0.016$ | $0.020 \pm 0.008$ |
| Framingham | $0.270 \pm 0.022$ | $0.124 \pm 0.018$ | $0.213 \pm 0.089$ | $0.117 \pm 0.067$ | $0.285 \pm 0.075$ | $0.136 \pm 0.038$ |
| MIMIC, mortality-gender | $0.050 \pm 0.012$ | $0.020 \pm 0.009$ | $0.072 \pm 0.018$ | $0.034 \pm 0.012$ | $0.018 \pm 0.011$* | $0.010 \pm 0.010$* |
| MIMIC, prolonged LOS-ethnicity | $0.043 \pm 0.008$ | $0.021 \pm 0.008$ | $0.034 \pm 0.012$ | $0.010 \pm 0.008$* | $0.025 \pm 0.010$ | $0.012 \pm 0.007$ |
| eICU, prolonged LOS-ethnicity | $0.088 \pm 0.018$ | $0.029 \pm 0.015$ | $0.076 \pm 0.017$ | $0.026 \pm 0.012$ | $0.083 \pm 0.029$ | $0.032 \pm 0.018$ |

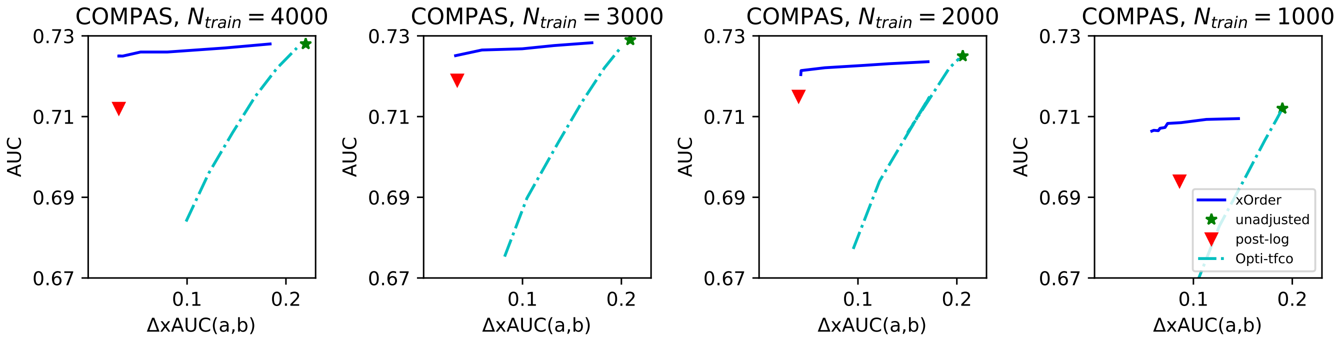


(a) Adult data set given fewer training samples(20000, 15000, 10000, 5000)

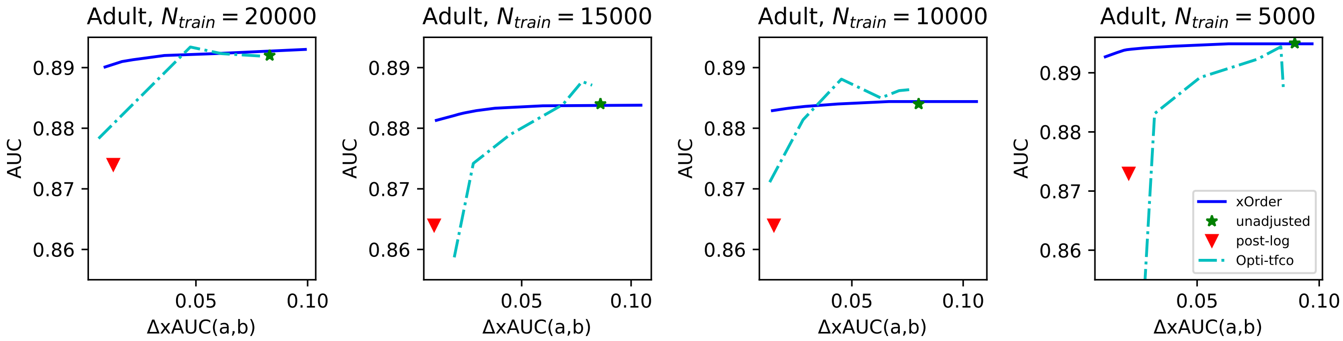


(b) COMPAS data set given fewer training samples(4000, 3000, 2000, 1000)

Fig. 1: AUC-ΔxAUC trade-offs using linear model optimizing AUC with fewer training samples on Adult and COMPAS

results on the Adult data set shown in Figure 1(b) also confirm the statement. As the number of training samples reduced to 5000, `xOrder` realizes the lowest disparity(ΔxAUC $= 0.01$) compared to baselines(ΔxAUC $= 0.02$). From the two series experiments on COMPAS and Adult, `xOrder` has stable performances on all experiments which maintain its advantages that realize a maximum algorithm utility and a minimum ranking disparity.

## IX. Distribution Shifts

As a post-processing algorithm, `xOrder` adjusts the ordering directly while post-logit transforms the ranking scores to reduce the disparity. To compare the robustness of the two algorithms when faced with the difference between training and test ranking score distributions, we implement experiments on two data sets with 2 base models (linear model and RankBoost) on ΔxAUC metric.

According to Figure 8, post-logit fails to achieve ΔxAUC as low as `xOrder` with bipartite rankboost model, while both methods can achieve low ΔxAUC with a linear model as shown in Figure 5. To analyze this phenomenon, we use COMPAS and Adult as examples in Figure 2 and 3. For different models, we illustrate the distributions of prediction scores S on training and test data. We further plot ΔxAUC on training data versus ΔxAUC on test data. With a linear model, the distributions of S on training and test data are close to each other. In this situation, the transform relations learned from post-logit and `xOrder` can both obtain results with low ΔxAUC on test data. While the distributions of the scores S on training and test data become significantly different, the function learned from post-logit may not be generalized well on test data to achieve low ΔxAUC. Similar results can be observed on the Adult data set in Figure 3. These phenomena occur in repeat experiments on both data sets. We guess the reason is that `xOrder` adjusts the relative ordering and it is more flexible than post-logit which optimizes a logistic class function. According to the experiments, `xOrder` is more robust to such distribution difference.

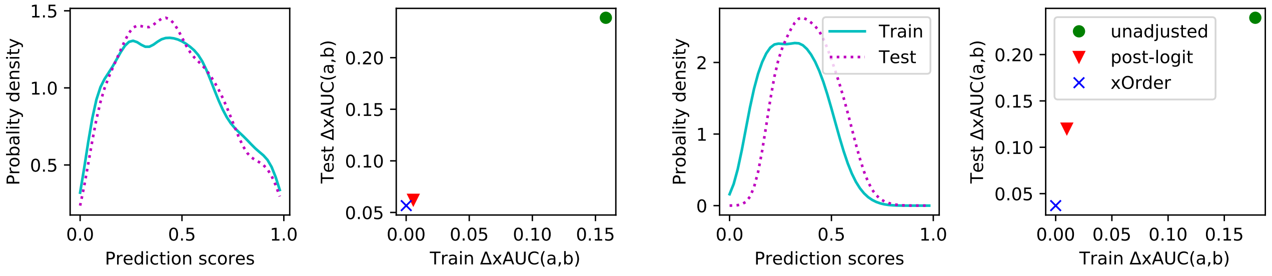


(a) (b)

Fig. 2: Result analysis on COMPAS data set with ΔxAUC metric. (a) illustrates the result with a linear model. (b) illustrates the result with a bipartite rankboost model. The left part of each sub-figure is the distribution of prediction scores on training and test data, and the right part of each sub-figure plots ΔxAUC on training data test data.

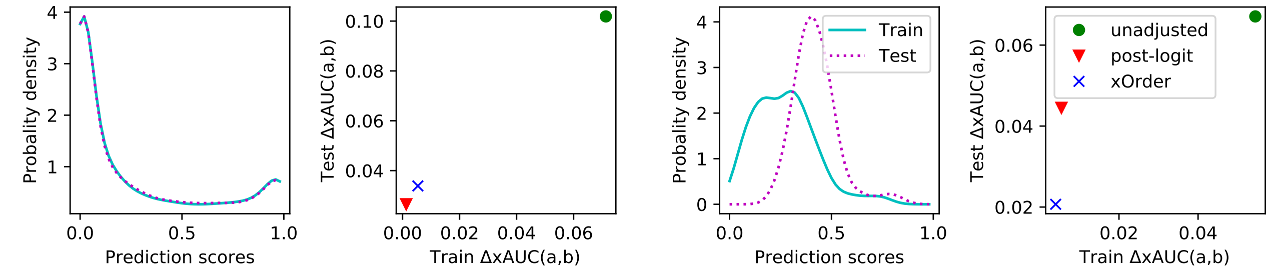


(a) (b)

Fig. 3: Result analysis on Adult data set with ΔxAUC metric. (a) illustrates the result with a linear model. (b) illustrates the result with a bipartite rankboost model. The left part of each sub-figure is the distribution of prediction scores on training and test data, and the right part of each sub-figure plots ΔxAUC on training data and test data.

## X. Additional Experiment Results

### A. *Ranking fairness analysis on unadjusted result*

We report the ranking fairness metrics($\Delta$xAUC, $\Delta$PRF) in Table IV. Large $\Delta$xAUC and $\Delta$PRF are observed on the five benchmark data sets. We use t-test with p-value as 0.0001 to evaluate whether the average $\Delta$xAUC and $\Delta$PRF do not equal to 0.We mark the results which do not pass the test with $*$ on the table. For MIMIC-III and eICU data set, disparities are significant with certain $\mathrm{Y}-\mathrm{A}$.

### B. *Complete experiment results*

The results with model-metric combinations of liner model-$\Delta$xAUC optimized by gradient descent, liner model-$\Delta$xAUC optimized by tfco, linear model-$\Delta$PRF optimized by gradient descent, linear model-$\Delta$PRF optimized by tfco, bipartite rankboost-$\Delta$xAUC and bipartite rankboost-$\Delta$PRF are shown in Figure 4, 5, 6, 7, 8 and 9 respectively. The source codes to reproduce these results on public data sets are at https://github.com/cuis15/xOrder. Most subfigures in Figure 5, 7 and 8 have been discussed in the main text.

## References


[1] H. Narasimhan, A. Cotter, M. R. Gupta, and S. Wang, "Pairwise fairness for ranking and regression." in *AAAI*, 2020, pp. 5248–5255.

[2] N. Kallus and A. Zhou, "The fairness of risk scores beyond classification: Bipartite ranking and the xauc metric," in *Advances in Neural Information Processing Systems*, 2019, pp. 3433–3443.

[3] S. A. Friedler, C. Scheidegger, S. Venkatasubramanian, S. Choudhary, E. P. Hamilton, and D. Roth, "A comparative study of fairness-enhancing interventions in machine learning," in *Proceedings of the conference on fairness, accountability, and transparency*, 2019, pp. 329–338.

[4] H. Harutyunyan, H. Khachatrian, D. C. Kale, G. Ver Steeg, and A. Galstyan, "Multitask learning and benchmarking with clinical time series data," *Scientific data*, vol. 6, no. 1, pp. 1–18, 2019.

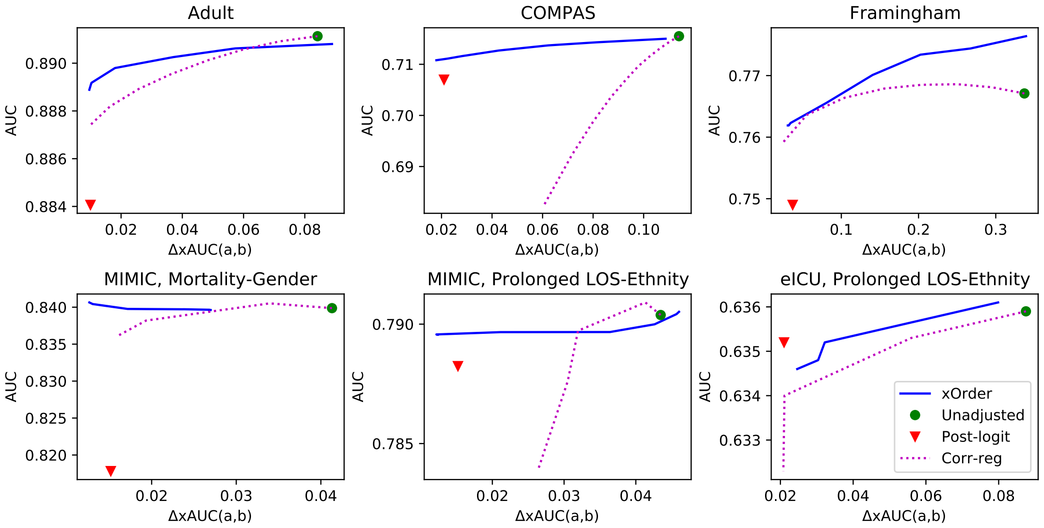


Fig. 4: AUC-ΔxAUC with linear model trained by gradient descent.

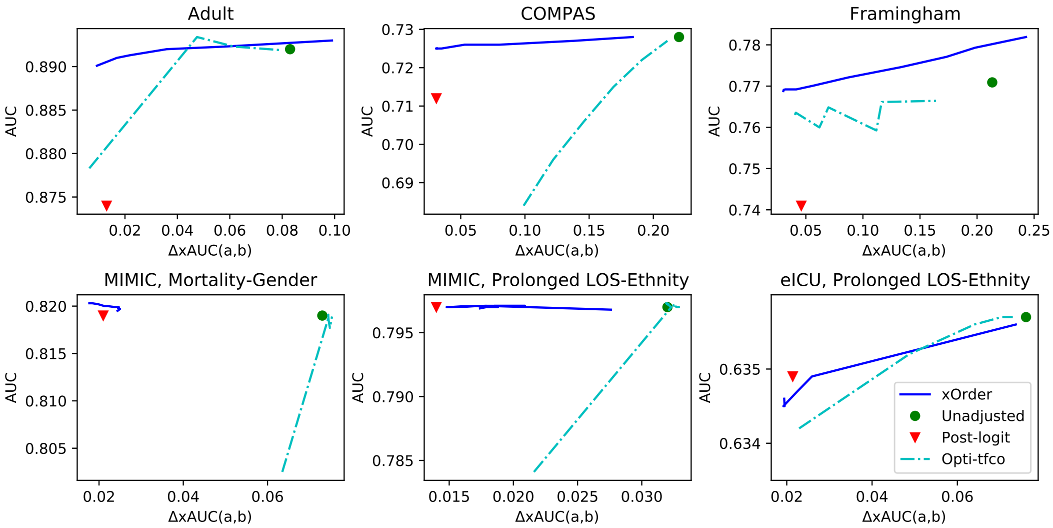


Fig. 5: AUC-ΔxAUC with linear model trained by tfco.

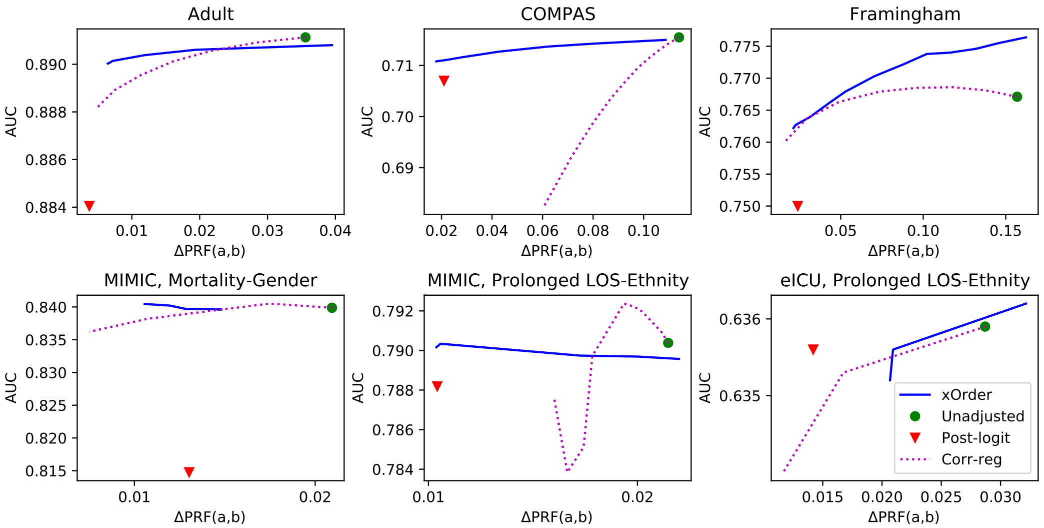


Fig. 6: AUC-ΔPRF with linear model trained by gradient descent.

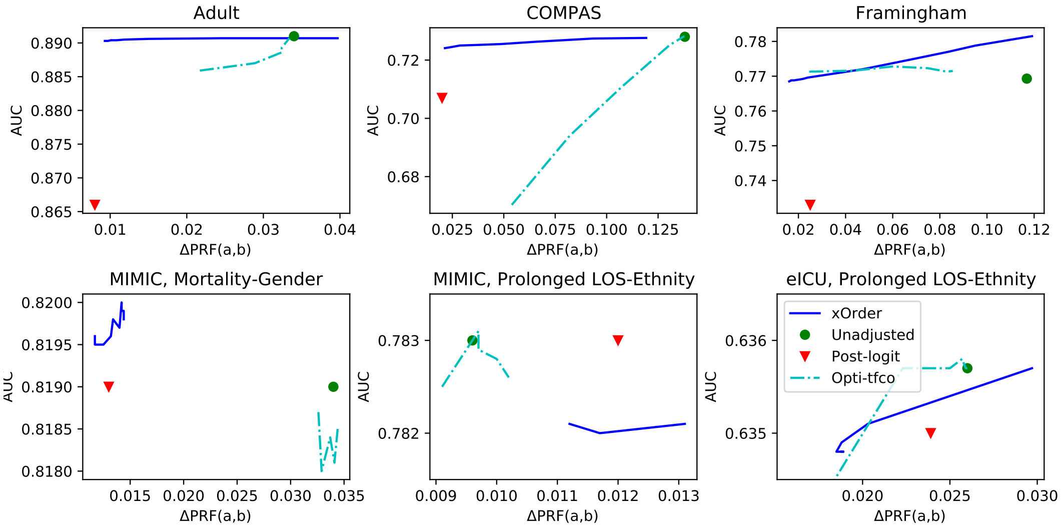


Fig. 7: AUC-ΔPRF with linear model trained by tfco.

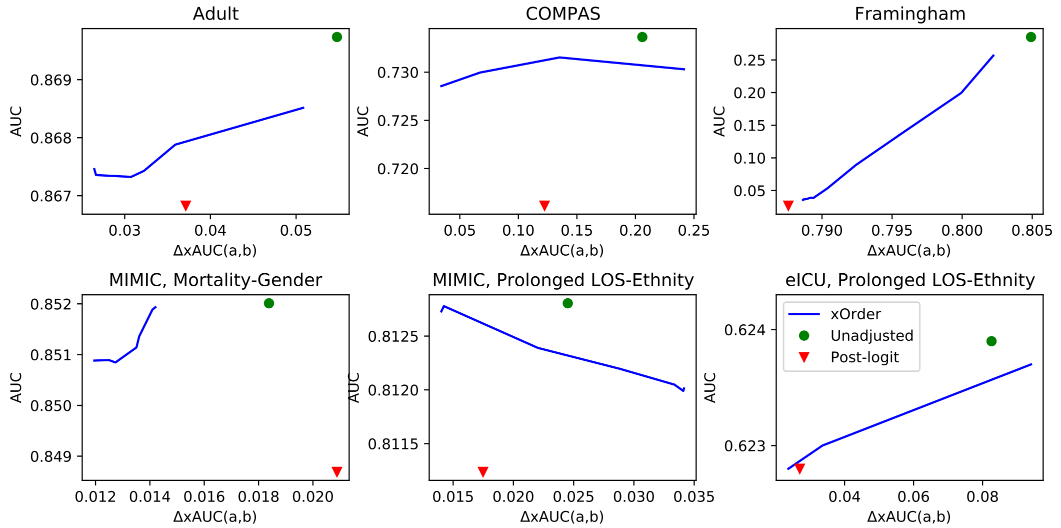


Fig. 8: AUC-ΔxAUC with bipartite rankboost model.

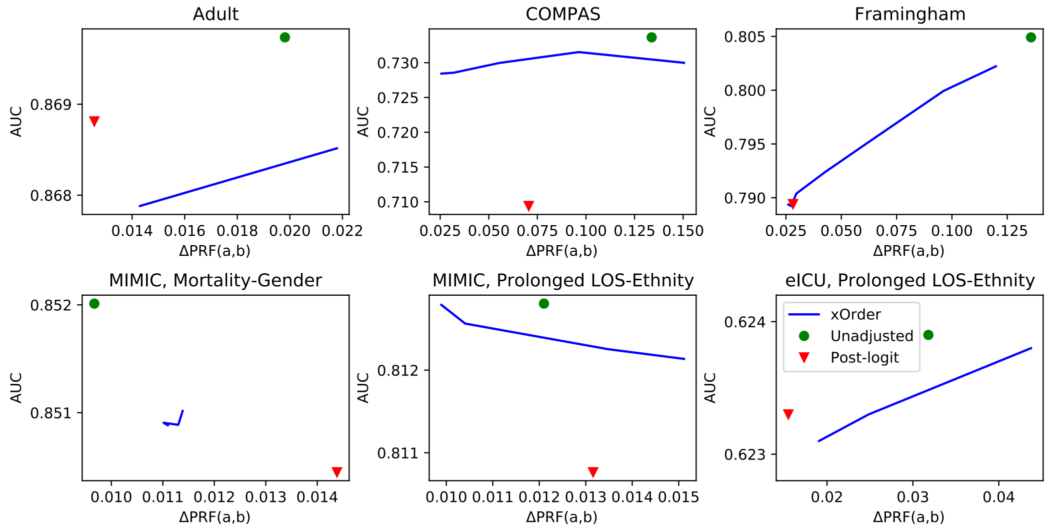


Fig. 9: AUC-ΔPRF with bipartite rankboost model.
